# Supplementary material for: Simulation and evaluation of sustainable climate trajectories for aviation
Source: arXiv:2102.01574 source file (2021-05-20)
Supplement: Supplementary file 1 [file article_appendix.tex]

\appendix

\section{Parameter setting for levers of action}
\label{parametersettinglevers}

\subsection{Efficiency} 

Tendanciel Croissance fixe
TABLEAU

\subsection{Load factor} 

Tendanciel Sigmoide
TABLEAU

\subsection{Other levers of action} 

Sigmoide
TABLEAU

\section{Parameter setting for scenarios}
\label{parametersettingscenarios}

Détail de tous les scénarios, comment introduire l'ensemble des variables ?
TABLEAU
